# Supplementary material for: FreeDNA: Endowing Domain Adaptation of Diffusion-Based Dense Prediction with Training-Free Domain Noise Alignment
Source: arXiv:2506.22509 source file (2025-06-26)
Supplement: Supplementary file 1 [file X_suppl.tex]

\clearpage
\setcounter{page}{1}
\setcounter{figure}{0}
\setcounter{table}{0}
\maketitlesupplementary

\setcounter{section}{0}

\section{More Implementation Details}
\label{sec:details}
\subsection{Dataset details}
\noindent\textbf{Depth Estimation.} We mainly test our Method on nuScenes and RobotCar datasets, both of which contain images on diverse conditions. nuScenes is a large autonomous driving dataset comprising 1000 video clips collected in diverse road scenes and weather conditions. These scenes are pretty challenging, with a fair amount of unexpected regions. RobotCar is a large-scale autonomous driving dataset including driving videos captured on a consistent route during various weather conditions, traffic conditions, and times of day and night. 

\noindent Morover, we also test our method on more commonly used dataset, like NYUv2 and KITTI. The NYUv2 dataset is a high-quality dataset widely used for depth estimation and indoor scene understanding, released by New York University. It contains 1,449 pairs of RGB-D images, captured from diverse indoor scenes (such as offices, living rooms, kitchens, etc.), with depth information acquired using the Microsoft Kinect sensor.
